# Supplementary material for: Calibration Is Not Enough: Evaluating Confidence Estimation Under Language Variations
Source: arXiv:2601.08064 source file (2026-09-23)
Supplement: Supplementary file 1 [file appendix.tex]

\subsection{Implementation Details}

\paragraph{Robustness.}
To evaluate robustness, we estimate confidence scores for the same answer under different prompt formulations. For GPT-4o, full input-sequence logits are not available, which prevents computing the probability of a fixed answer across prompts. We therefore compute confidence based on the generated output sequences instead. Note that this might bring minor changes in the overall robustness results for Prob. method, it does not impact our overall findings.

\paragraph{Stability and Sensitivity.}
We set the LLM temperature to 0.7 to generate diverse candidate answers. GPT-4o is used as a judge model to assess semantic equivalence and group answers accordingly.

\paragraph{CE Methods.}
For Calib-1, we follow the setup of \citet{xia-etal-2025-influences}, using BERT-base-uncased as the backbone model for training.

\subsection{Technical Details}
We use the vLLM \cite{vllm2023} library for LLM inference and serving, the temperature of all LLMs is set to 0 for greedy-encoding model outputs.  All our experiments are conducted on NVIDIA HGX H100, which requires approximately 600 GPU hours to replicate.
\input{tables/answer_prompt_table}
\input{tables/prompts_table}

\input{tables/stability_table}
% \input{tables/overall_metric_table}
% \input{tables/new_detailed_results}
% \input{tables/ov_cali_table}

% For example,  Fig. \ref{fig:corr_olmo_model} demonstrates the low correlation of RP(1) and  RP(\%) prompts (explained in Table \ref{tab:prompt_detail}) to other prompts on different sizes of OLMo models.

% \textbf{Larger models generally generate more stable VC.} The consistency of all models in Table \ref{tab:stability} demonstrates that larger models (>70B parameters) provide more consistent confidence than smaller models. Similarly, scores of Qwen models show that consistency is correlated with model size--larger models are more consistent. However, this does not apply to OLMo models, where OLMo-32B INS is less consistent than both OLMo-13B and -7B models. We hypothesize that OLMo models can vary in performance due to their different post-training data, which may impact their complex reasoning capability.

\subsection{Robustness:  Confidence-elicit Prompts for Verbalized Conf.}\label{sec:conf-prompt-vc}

To evaluate robustness, we design seven variants of the confidence-elicitation prompt (see Appendix, Table~\ref{tab:prompt_detail}), grouped into three types:
(i) Scale variants, which elicit confidence using numerical ranges of 0–1, 0–100\%, and 0–10;
(ii) Lexical variants, which vary the key term used to request a score between 0 and 1 (``probability'', ``certainty'' and ``confidence''); and
(iii) Linguistic expressions, following \citet{tian2023just}, which elicit confidence using predefined verbal scales from ``Almost No Chance'' to ``Almost certain'', and a corresponding multiple-choice format (e.g., ``a: Almost No Chance'').
Those selected expressions are converted to numerical scores according to rules in \cref{prompt_detail}.
All confidence outputs are normalized to a 0–1 scale for comparison.

\paragraph{Mapping of Linguistic Prompts.} For the linguistic prompts, we followed \citet{tian2023just} to map the linguistic expressions to numerical scores. The specific mapping are [``Almost No Chance'', ``Highly Unlikely'', ``Chances are Slight'',
``Little Chance'', ``Unlikely'', ``Probably Not'', ``About Even'', ``Better than Even'',
``Likely'', ``Probably'', ``Very Good Chance'', ``Highly Likely'', ’Almost Certain''] to [0.02, 0.05, 0.1, 0.1, 0.2, 0.25, 0.5, 0.6, 0.7, 0.7, 0.8, 0.9, 0.95] according to \citet{fagen-ulmschneider2023perception}.
We further conducted an experiment applying \textbf{VC} using only the answer-elicit prompts to examine how confidence values change under this setting. This design allows us to isolate the influence of answer-elicit prompts on VC and directly compare it with the other two methods under consistent perturbation conditions, even though the confidence-elicit prompt is expected to have a more direct effect on VC. As shown in Table~\ref{tab:ans-conf-vc}, when using answer-elicit prompts (Ans-P), VC produces more stable confidence estimates ($\text{P-RB}=0.968$) compared to when confidence-elicit prompts are used ($\text{P-RB}=0.904$). We hypothesize that this improvement in stability arises because the generated answers remain largely consistent across perturbed answer-elicit prompts, leading to nearly identical instructions when subsequently eliciting confidence for those answers. In contrast, perturbations to the confidence-elicit prompts directly alter how the model is instructed to express its confidence, thereby introducing greater variability in the resulting confidence scores.

\paragraph{Prompt-wise Confidence Analysis for VC.}
We examine the pairwise correlations of confidences between prompts for individual models (shown by Fig. \ref{fig:corr_large_model}-\ref{fig:corr_olmo_model}). We found that larger models maintain higher stability of confidence, demonstrating their ability to respond to diverse confidence-eliciting prompts.  

\textbf{LLMs remain stable with the change of scales and lexical words in prompts}. Fig. \ref{fig:corr_large_model}-\ref{fig:corr_olmo_model}) shows that prompts of only scale and lexical words change tend to have more correlated verbalized confidence compared to adding linguistic expressions in the prompt. Small models (<= 32B) struggle more in maintaining stability, especially with the multi-choice linguistic expression prompts. 

\subsection{Sensitivity: Alternative Sets of Semantically Different Answers}\label{sec:sens_add}

Table~\ref{tab:sens_add} reports sensitivity results obtained by using all semantically different answers outside $\hat{\mathcal{Y}}^{\text{max}}$ (denoted as $\hat{\mathcal{Y}}^{\notin \text{max}}$), instead of the original setting that compares $\hat{\mathcal{Y}}^{\text{max}}$ with $\hat{\mathcal{Y}}^{\text{min}}$. The results remain stable under this alternative definition and do not affect the main findings of the paper.

\begin{table*}[t]
\centering
\setlength{\tabcolsep}{5pt}
\footnotesize
\begin{tabular}{llllllll}
\toprule
CE & P-RB $\uparrow$ & A-STB $\uparrow$ & A-SST $\uparrow$ & Brier $\downarrow$ & AUROC $\uparrow$ & ECE $\downarrow$ & smECE $\downarrow$ \\
\midrule
BL       & 0.728 & 0.748 & 0.087 & 0.335 & 0.486 & 0.288 & 0.229 \\
Prob.    & 0.949 & 0.959 & 0.208 & 0.275 & 0.678 & 0.264 & 0.227 \\
PS       & 0.990 & 0.991 & 0.046 & 0.216 & 0.649 & 0.076 & 0.043 \\
VC       & 0.945 & 0.985 & 0.105 & 0.262 & 0.701 & 0.258 & 0.209 \\
P(True)  & 0.976 & 0.987 & 0.219 & 0.296 & 0.733 & 0.295 & 0.171 \\
Calib1   & 0.982 & 0.977 & 0.087 & 0.208 & 0.704 & 0.104 & 0.103 \\
\bottomrule
\end{tabular}
\caption{GPT-4o results extracted from the detailed overall results table.}
\label{tab:gpt4o_results}
\end{table*}

\begin{figure*}[h]
    \centering
    \includegraphics[width=1\linewidth]{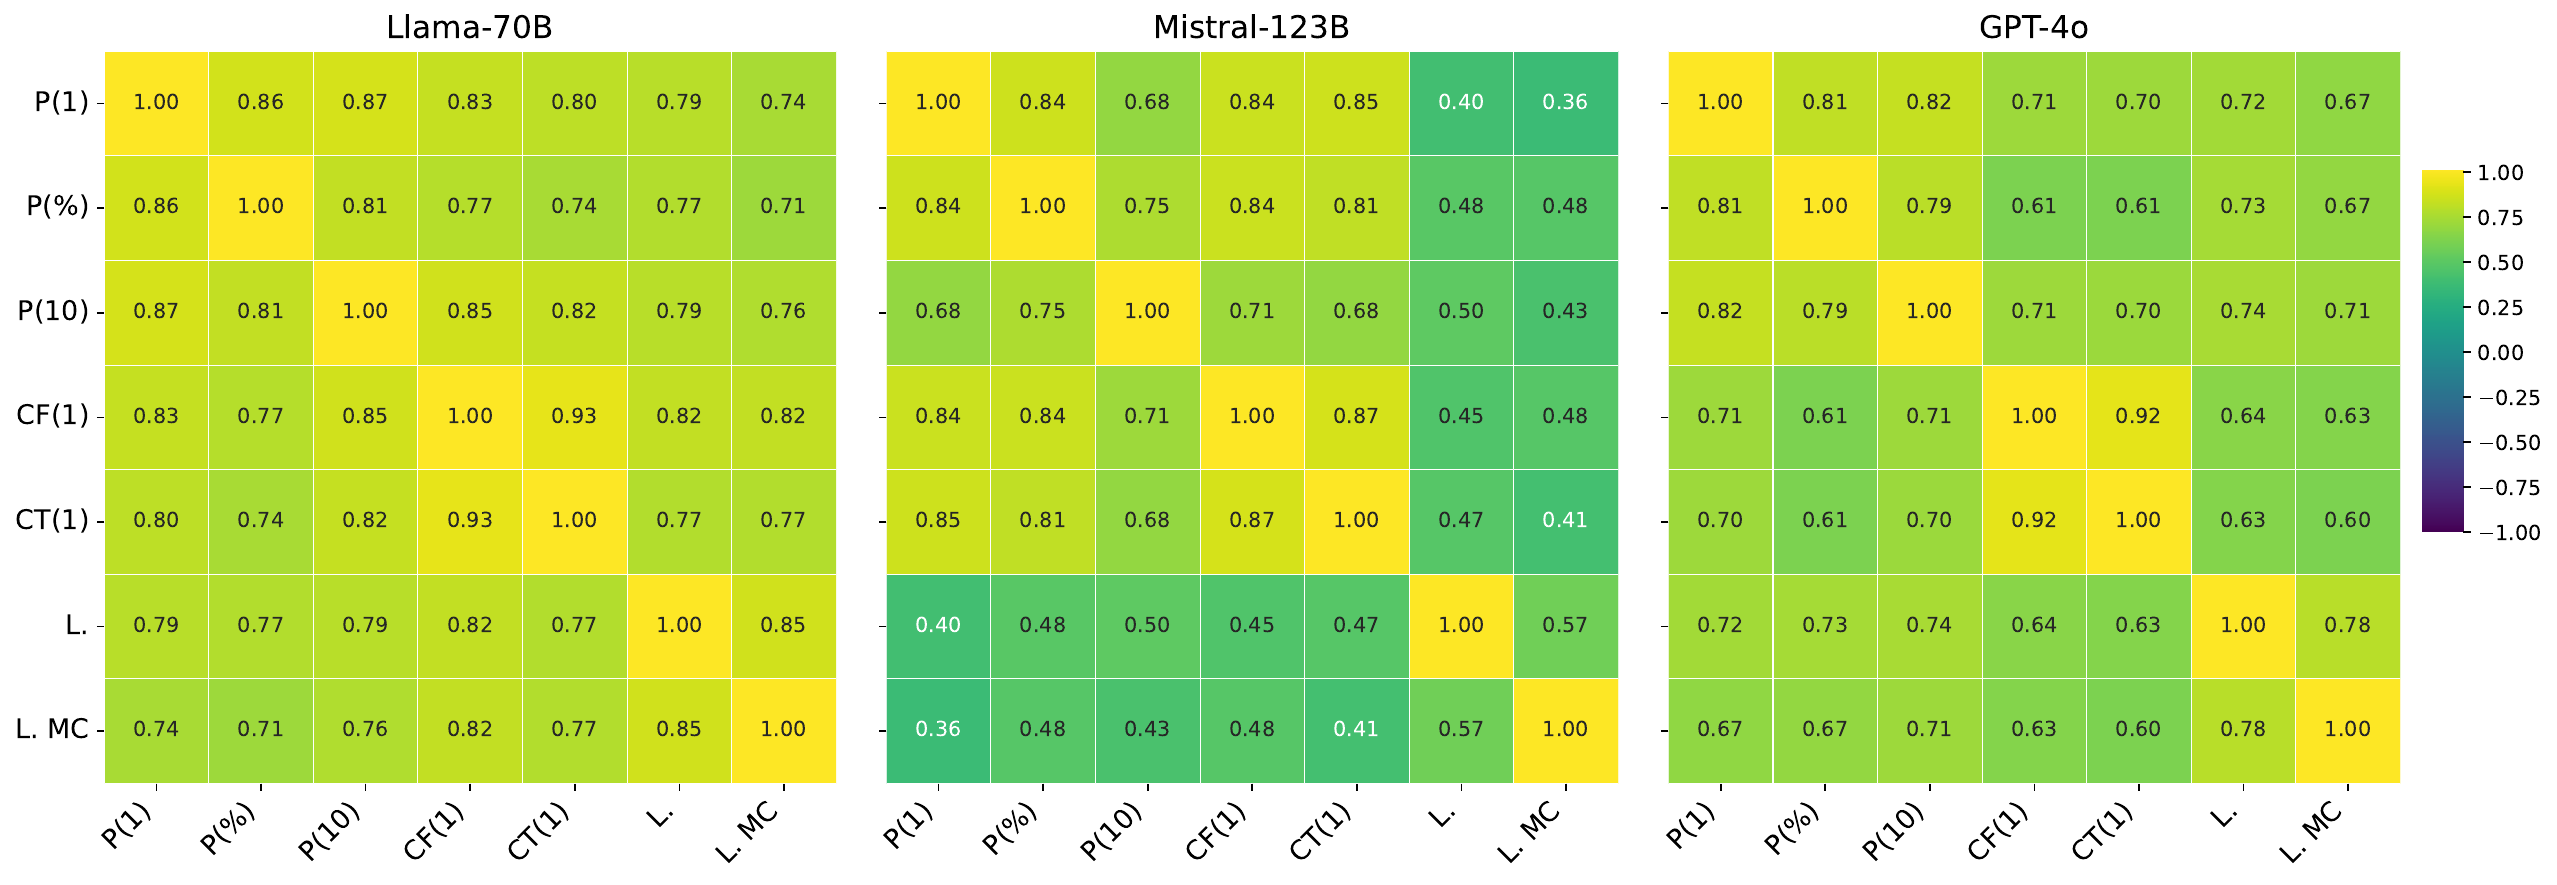}
    \caption{\textit{Robustness}: Pearson correlations of VC when using different prompts on large models from different model families.}
    \label{fig:corr_large_model}
\end{figure*}

\begin{figure*}[h]
    \centering
    \includegraphics[width=1\linewidth]{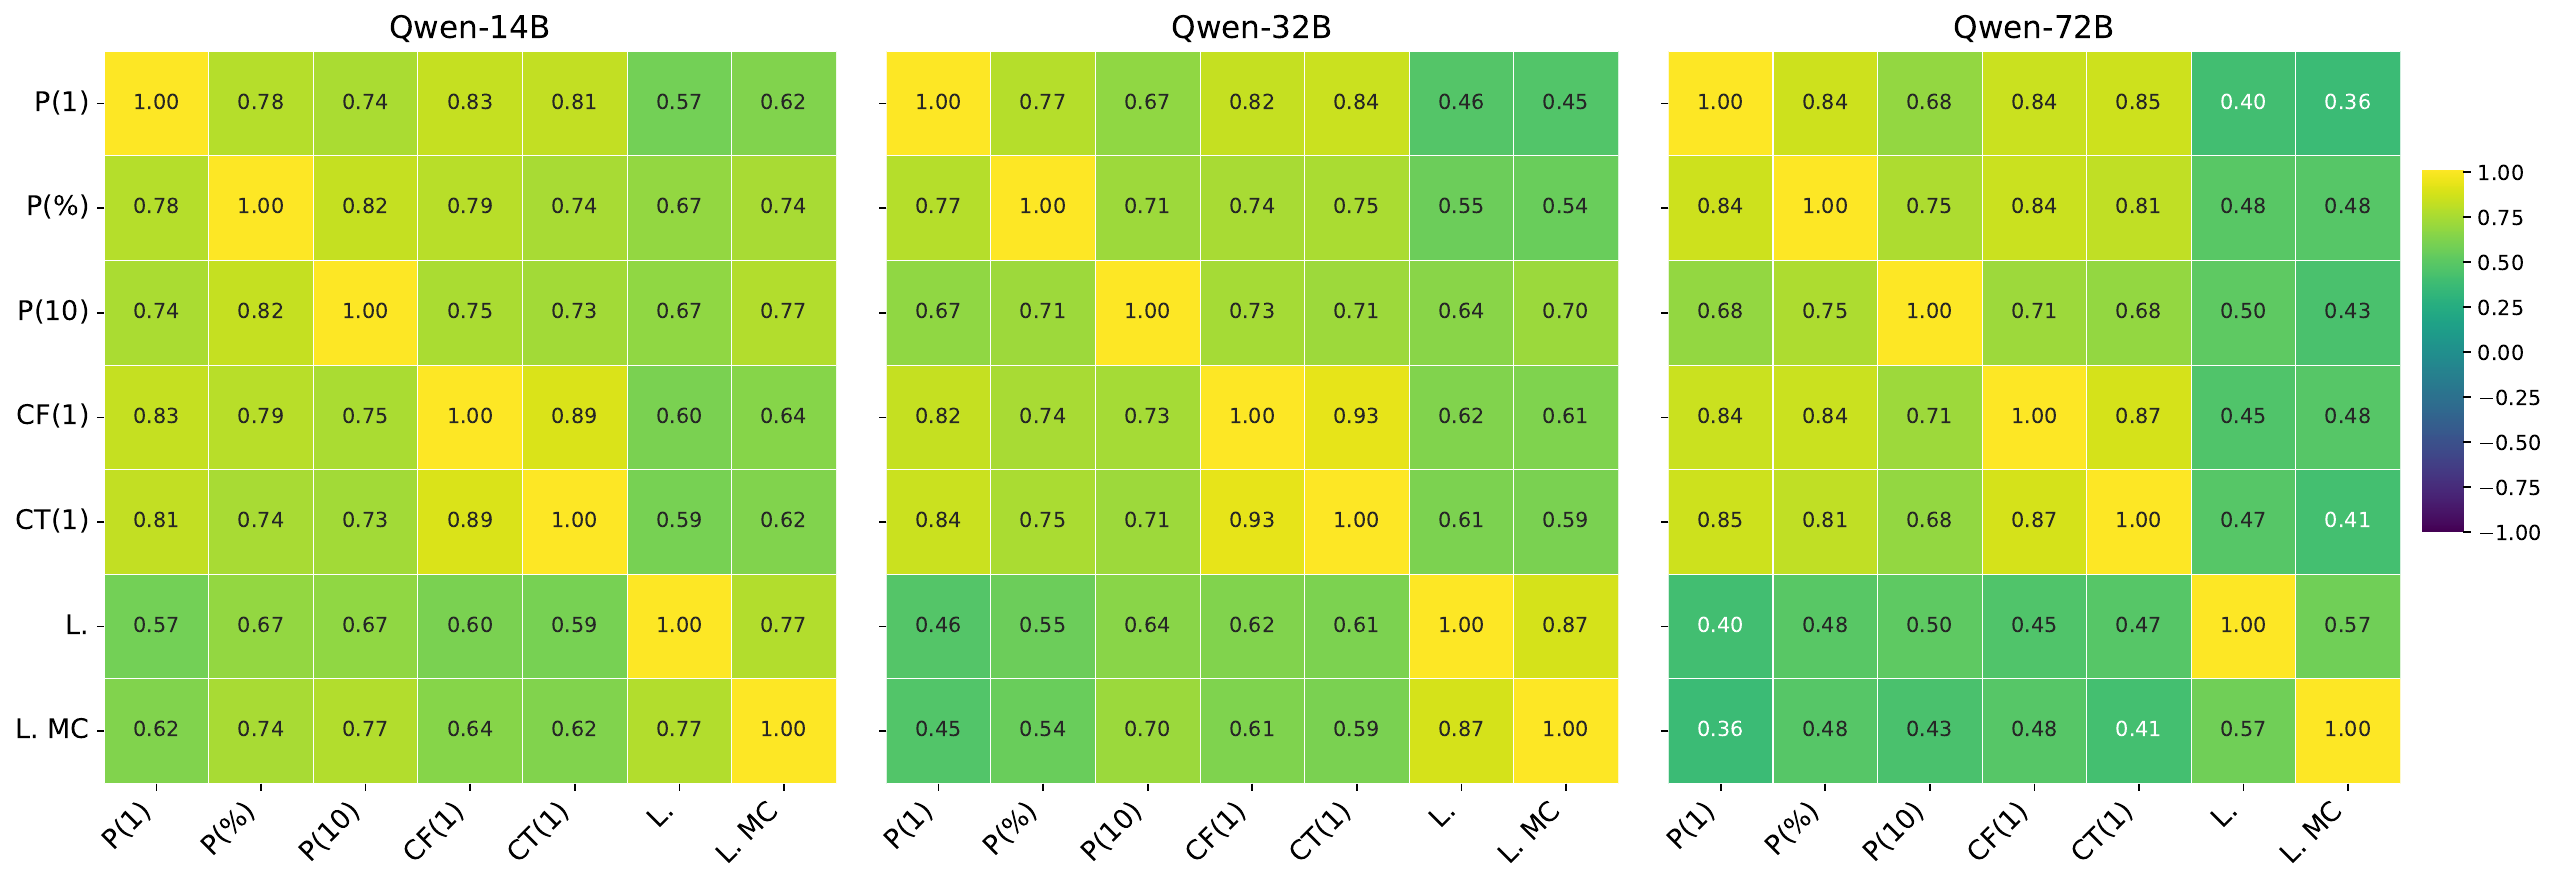}
    \caption{\textit{Robustness}:  Pearson correlations of VC when using different prompts on Qwen models with different sizes.}
    \label{fig:corr_qwen_model}
\end{figure*}

\begin{figure*}[h]
    \centering
    \includegraphics[width=0.95\linewidth]{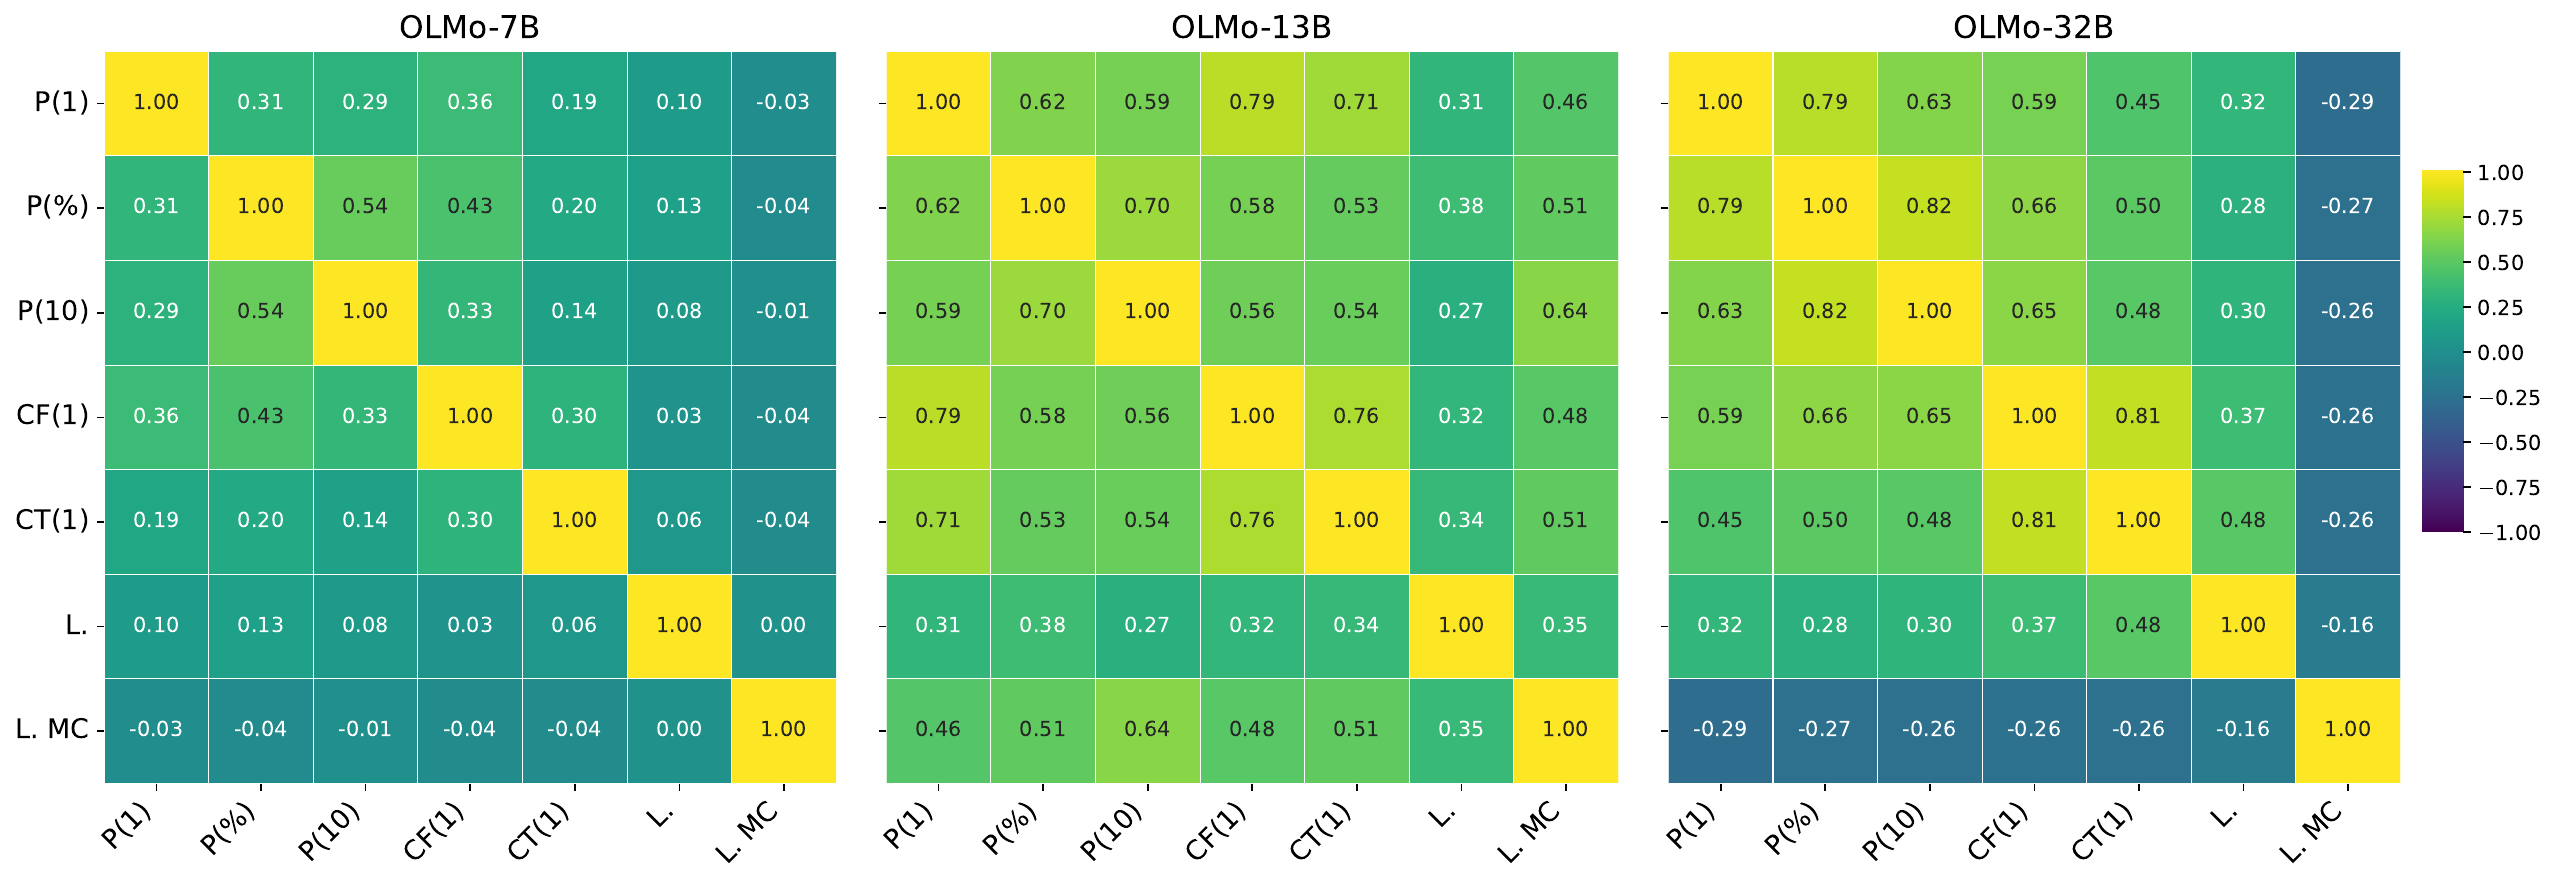}
    \caption{\textit{Robustness}:  Pearson correlations of VC when using different prompts on OLMo models with different sizes.}
    \label{fig:corr_olmo_model}
\end{figure*}

% \begin{figure*}[h]
%     \centering
%     \includegraphics[width=1\linewidth]{analysis_plots/consistency/13b_ft_scheme_consistency.pdf}
%     \caption{\textit{Stability}: Pearson correlations of prompts in VC on OLMo-13B models with different fine-tuning schemes.}
%     \label{fig:corr_olmo13b_ft}
% \end{figure*}

% \begin{figure*}[htbp]
%     \centering
%     \includegraphics[width=1\linewidth]{analysis_plots/consistency/7b_ft_scheme_consistency.pdf}
%     \caption{Stability: Pearson correlations of prompts in VC on OLMo-7B models with different fine-tuning schemes.}
%     \label{fig:corr_olmo7b_ft}
% \end{figure*}

% \begin{figure}[ht]
%     \centering
%      \begin{subfigure}[b]{0.48\textwidth} \includegraphics[width=\textwidth]{analysis_plots//overall/model_bar.pdf}
%      \caption{Mean fidelity and reliability of all instruction models over all prompts. Stability is measured on all prompts (same values as the \textbf{All} column in Table \ref{consistency_table}).   }
%     \end{subfigure}
%         \begin{subfigure}[b]{0.48\textwidth}
% \includegraphics[width=\textwidth]{analysis_plots//overall/prompt_bar.pdf}
% \caption{Prompt formatting matters: Mean influences of prompt types on fidelity and reliability evaluation and further averaged over all instruction models. Stability is measured on prompts in each type and averaged over all instruction models. }
%     \end{subfigure}
%      \caption{Overview of the main evaluation results. }
%     \label{fig:overall}
% \end{figure}

\begin{table*}
\centering
\scriptsize
\setlength{\tabcolsep}{3pt}
\begin{tabular}{llcrrrrrrrrrrr}
\toprule
\multicolumn{14}{c}{The electrode at which oxidation occurs is called?  ~$y$: the anode. ~Corr.: 1.00} \\
\midrule
\textbf{}& \textbf{} & \textbf{CE}& \textbf{$t_1$} & $t_2$  & $t_3$  & $t_4$ & $t_5$ & $t_6$  & $t_7$  & $t_8$  &$t_9$ &$t_{10}$ & \textbf{P-RB}\\
\cmidrule(lr){1-3} \cmidrule(lr){4-13} \cmidrule(lr){14-14}
\multirow{10}{*}{ \rotatebox[origin=c]{90}{Qwen-14B} } & \multirow{10}{*}{ \rotatebox[origin=c]{90}{SciQ} } & Seq. Likelihood & 0.96 & 0.72 & 0.98 & 1.00 & 1.00 & 1.00 & 0.99 & 0.89 & 1.00 & 1.00 & 0.92 \\
 &  & Boosted Prob. & 1.00 & 1.00 & 1.00 & 1.00 & 1.00 & 1.00 & 1.00 & 1.00 & 1.00 & 1.00 & 1.00 \\
 &  & Platt Scaling & 0.75 & - & 0.75 & 0.75 & 0.75 & 0.75 & 0.75 & 0.73 & 0.75 & 0.75 & 0.99 \\
 &  & P(True) & 1.00 & 1.00 & 0.00 & 0.00 & 1.00 & 1.00 & 0.00 & 1.00 & 0.00 & 0.00 & 0.50 \\
 &  & Calib1 & 0.77 & 0.76 & 0.77 & 0.76 & 0.76 & 0.78 & 0.77 & 0.75 & 0.74 & 0.76 & 0.99 \\
 &  & Verbalized Conf. & 0.95 & 0.95 & 0.95 & 0.95 & 0.95 & 0.95 & 0.95 & 0.95 & 0.95 & 0.95 & 1.00 \\
 &  & Hidden Score & 0.85 & 0.86 & 0.84 & 0.84 & 0.83 & 0.86 & 0.84 & 0.85 & 0.83 & 0.83 & 0.99 \\
 &  & Attention Score & 0.81 & 0.81 & 0.80 & 0.81 & 0.81 & 0.81 & 0.80 & 0.80 & 0.81 & 0.81 & 1.00 \\
 &  & SAPLMA & 1.00 & 1.00 & 1.00 & 0.99 & 0.99 & 1.00 & 1.00 & 1.00 & 0.99 & 0.98 & 0.99 \\
 &  & P(IK) & 0.90 & 0.89 & 0.88 & 0.91 & 0.91 & 0.91 & 0.89 & 0.89 & 0.93 & 0.95 & 0.98 \\
\bottomrule
\end{tabular}
\caption{Case study of prompt robustness. The confidence estimated by different CE methods under 10 perturbed prompts for the same question and LLM response is shown.}
\label{tab:case-robust-detail}
\end{table*}

\begin{table*}
\centering
\scriptsize
\setlength{\tabcolsep}{3pt}
\begin{tabular}{lllrrrr}
\toprule
\multicolumn{7}{c}{In what country is Gregory? ~~ $y^*$: Australia} \\
 &  &  & United States & The question does not... &  &  \\
\midrule
& & CE & $y_{1}$ & $y_{2}$ & \textbf{A-STB} & \textbf{A-SST} \\
\cmidrule(lr){1-3} \cmidrule(lr){4-5} \cmidrule(lr){6-7}
\multirow{10}{*}{\rotatebox[origin=c]{90}{qwen32b} } & \multirow{10}{*}{ \rotatebox[origin=c]{90}{PopQA} } & Seq. Likelihood & 0.59 & 0.93 & 1.00 & 0.34 \\
 &  & Boosted Prob. & 0.99 & 1.00 & 1.00 & 0.00 \\
 &  & Platt Scaling & 0.52 & 0.59 & 1.00 & 0.06 \\
 &  & P(True) & 0.00 & 1.00 & 1.00 & 1.00 \\
 &  & Calib1 & 0.65 & 0.57 & 1.00 & 0.08 \\
 &  & Verbalized Conf. & 0.00 & 1.00 & 1.00 & 1.00 \\
 &  & Hidden Score & 0.21 & 0.11 & 1.00 & 0.09 \\
 &  & Attention Score & 0.19 & 0.30 & 1.00 & 0.11 \\
 &  & SAPLMA & 0.98 & 0.00 & 1.00 & 0.98 \\
 &  & P(IK) & 0.46 & 0.46 & 1.00 & 0.00 \\
\bottomrule
\end{tabular}
\caption{Case study of answer stability and sensitivity. The confidence estimated by different CE methods for 10 sampled answers to the same question, using the same prompt, is shown.}
\label{tab:case-stab-sens-detail}
\end{table*}

\input{tables/dataset_tables}

% \input{tables/fidelity_table}

% \subsection{Calibration: Results of More Evaluation Metrics}\label{reliability}

% To provide a robust evaluation of calibration, we followed \cite{ulmer-etal-2024-calibrating} and tested all the prompts and models with three more calibration metrics: ECE, smECE and AUROC. The results are shown in Table \ref{tab:detailed_results}.

\section{Case study}
